# Supplementary material for: Suppression of atomic displacive excitation in photo-induced A$_{\mathrm{1g}}$ phonon mode of bismuth unveiled by low-temperature time-resolved x-ray diffraction
Source: arXiv:2105.13146 source file (2022-11-30)
Supplement: Supplementary file 1 [file Bi_SM_arXivsubmit.pdf]

Supplementary material

# Suppression of atomic displacive excitation in photo-induced $A_{1g}$ phonon mode of bismuth unveiled by low-temperature time-resolved x-ray diffraction

Yuya Kubota[1,*], Yoshikazu Tanaka[1], Tadashi Togashi[2,1], Tomio Ebisu[1], Kenji Tamasaku[1], Hitoshi Osawa[2], Tetsuya Wada[3], Osamu Sugino[3], Iwao Matsuda[3], and Makina Yabashi[1,2]

[1]*RIKEN SPring-8 Center, 1-1-1 Kouto, Sayo, Hyogo 679-5148, Japan*

[2]*Japan Synchrotron Radiation Research Institute (JASRI),1-1-1 Kouto, Sayo, Hyogo 679-5198, Japan*

[3]*Institute for Solid State Physics, The University of Tokyo, Kashiwa, Chiba 277-8581, Japan*

We also measured the photo-induced coherent phonon of bismuth (Bi) at room temperature (RT) with absorbed excitation fluence of 1.2 mJ/cm$^2$ using the same sample as described in the main text. The optical laser was focused to ~1.2 mm in diameter (full-width-at-half-maximum, FWHM). The angle between the optical laser and the XFEL beams was 3.7 degrees. Other experimental parameters were the same as described in the main text. Figure S1 shows a result of the Bi 111 diffraction intensity variation as a function of the delay time ($t$) associated with the $A_{1g}$ coherent phonon mode at RT. The analysis was performed using the same method as for $T = 9$ K. Figure S2 shows the values of frequency and $\Delta x$ taken at RT (1.2 mJ/cm$^2$) as well as by the previous work at RT (Ref. [23] in the main text). We evaluated $\Delta x$ at RT with the same method as described in the main text and used the equilibrium values of $x(0)$ and $c$ before a photo-excitation at RT as 0.46719 and 11.8 Å, respectively [23]. The results at RT match with each other and confirm the validity of our comparison in Fig. 3 in the main text.

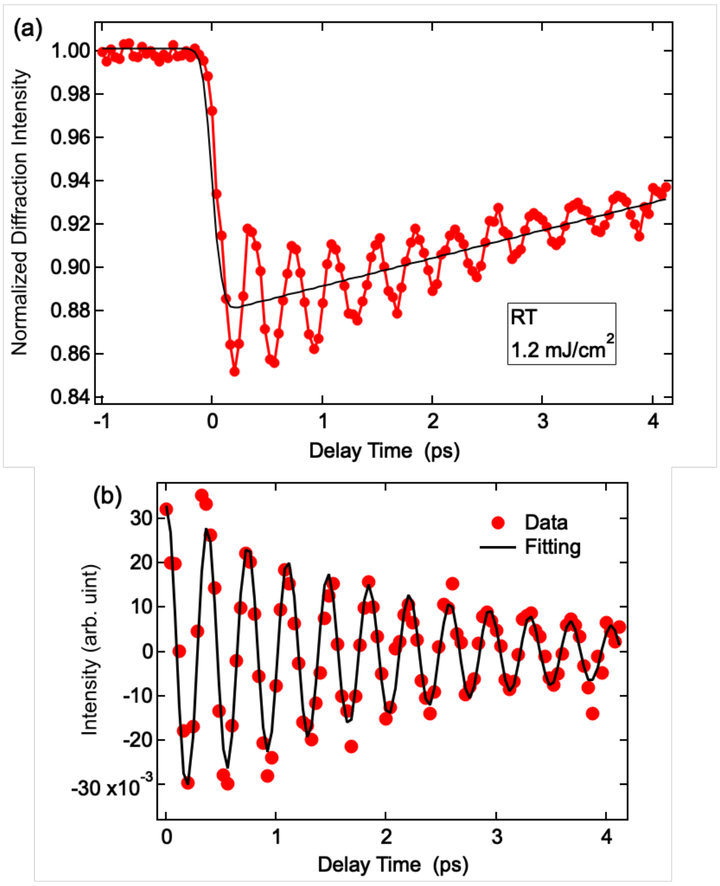


FIG. S1. (a) Bi 111 diffraction intensity variation as a function of the delay time obtained at RT and fluence of 1.2 mJ/cm$^2$, shown as the red circles. The red line is a guide to the eye. The black solid line represents a fitting curve of the non-oscillatory component with an exponential decay function convoluted with a Gaussian function. (b) Oscillatory component obtained by subtracting the non-oscillatory component from (a), shown as the red circles. The black solid line represents a fitting exponentially decaying cosine curve.

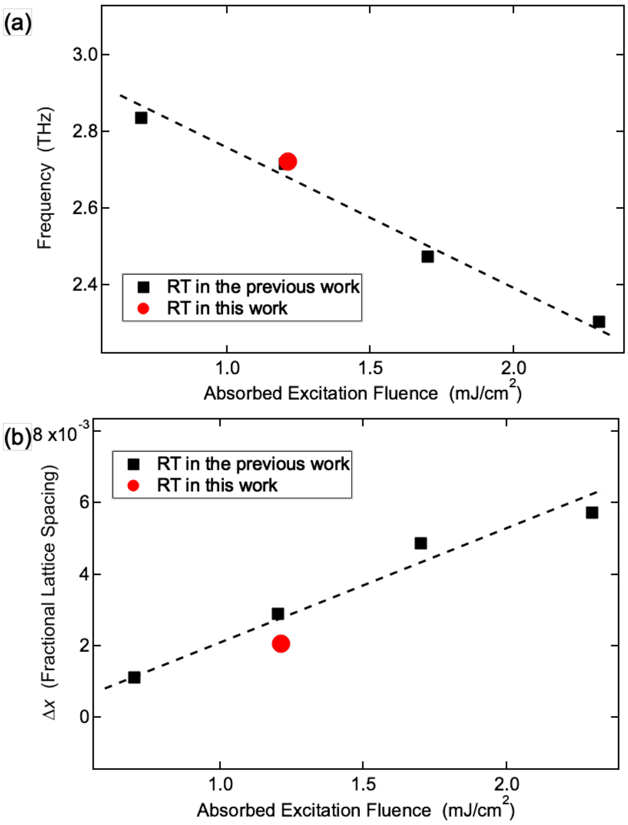


FIG. S2. (a) Frequency of the $A_{1g}$ phonon mode and (b) the atomic displacement $\Delta x$ as a function of absorbed excitation fluence. The red circles represent our data at RT, while the black squares and the dashed lines are the same as shown in Fig. 3 in the main text.
